# Supplementary material for: Multimodal Distillation for Egocentric Action Recognition
Source: arXiv:2307.07483 source file (2023-07-18)
Supplement: Supplementary file 1 [file supplementary-tables.tex]

% TODO: Needs to be pruned

\begin{table*}[t]
\begin{subtable}[t]{0.46\textwidth}
\centering
\resizebox{\columnwidth}{!}{
\begin{tabular}{>{\columncolor{graygray}}c>{\columncolor{pinkpink}}c>{\columncolor{yellowyellow}}c>{\columncolor{graygray}}c>{\columncolor{greengreen}}c>{\columncolor{greengreen}}c>{\columncolor{greengreen}}c} \toprule
    % {} & {} & \multicolumn{2}{|c|}{TT augmentation} & \multicolumn{3}{|c|}{Epic-100} \\
    {Method} & {Training modalities} & {Inference Modalities} & {Views} & {Noun} & {Verb} & {Action} \\ \midrule
    Baseline & RGB & RGB & 1x1 & 52.0 & 61.7 & 38.3 \\ \midrule \midrule
    Modality specific & OF & OF & 1x1 & 34.1 & 59.0 & 25.9 \\
    Teacher & \NA & RGB \& OF & 1x1 & 51.9 & 65.3 & 39.5 \\
    Student & RGB \& OF & RGB & 1x1 & 52.2\textsubscript{\textcolor{redred}{\textbf{+0.2}}} & 65.6\textsubscript{\textcolor{redred}{\textbf{+3.9}}} & 39.9\textsubscript{\textcolor{redred}{\textbf{+1.6}}} \\ \midrule
    Modality specific & A & A & 1x1 & 22.3 & 46.5 & 15.1 \\
    Teacher & \NA & RGB \& A & 1x1 & 52.7 & 64.4 & 39.8 \\
    Student & RGB \& A & RGB & 1x1 & 51.5\textsubscript{\textcolor{redred}{\textbf{-0.5}}} & 62.4\textsubscript{\textcolor{redred}{\textbf{+0.7}}} & 37.9\textsubscript{\textcolor{redred}{\textbf{-0.4}}} \\ \midrule
  Teacher & \NA & RGB \& OF \& A & 1x1 & X & X & X \\
    Student & RGB \& OF \& A & RGB & 1x1 & 51.7\textsubscript{\textcolor{redred}{\textbf{-0.3}}} & 65.4\textsubscript{\textcolor{redred}{\textbf{+3.7}}} & 39.3\textsubscript{\textcolor{redred}{\textbf{+1.0}}} \\ \midrule \midrule \midrule
    Baseline & RGB & RGB & 3x4 & 54.2 & 63.7 & 40.2 \\ \midrule
    Modality specific & OF & OF & 3x4 & 36.2 & 61.4 & 27.2 \\
    Teacher & \NA & RGB \& OF & 3x4 & 53.3 & 66.6 & 40.9 \\
    Student & RGB \& OF & RGB & 3x4 & 52.5\textsubscript{\textcolor{redred}{\textbf{-1.7}}} & 65.6\textsubscript{\textcolor{redred}{\textbf{+1.9}}} & 39.6\textsubscript{\textcolor{redred}{\textbf{-0.6}}} \\ \midrule
    Baseline & RGB & RGB & 1x4 & 53.7 & 63.6 & 39.8 \\ \midrule \midrule
    Modality specific & A & A & 1x4 & 23.1 & 48.4 & 15.8 \\
  Teacher & \NA & RGB \& A & 1x4 & 53.9 & 66.1 & 41.2 \\
    Student & RGB \& A & RGB & 1x4 & 53.1\textsubscript{\textcolor{redred}{\textbf{-0.6}}} & 63.8\textsubscript{\textcolor{redred}{\textbf{+0.2}}} & 39.1\textsubscript{\textcolor{redred}{\textbf{-0.7}}} \\ \midrule
    Teacher & \NA & RGB \& OF \& A & 1x4 & X & X & X \\
    Student & RBG \& OF \& A & RGB & 1x4 & 52.9\textsubscript{\textcolor{redred}{\textbf{-0.8}}} & 66.6\textsubscript{\textcolor{redred}{\textbf{+3.0}}} & 40.3\textsubscript{\textcolor{redred}{\textbf{+0.5}}} \\ \bottomrule
\end{tabular}
}
\caption{Epic-Kitchens \cite{damen2020rescaling} regular active object (noun) and activity (verb) recognition.}
\end{subtable}
\hfill
\begin{subtable}[t]{0.48\textwidth}
\centering
\resizebox{\columnwidth}{!}{
\begin{tabular}{>{\columncolor{graygray}}c>{\columncolor{pinkpink}}c>{\columncolor{yellowyellow}}c>{\columncolor{graygray}}c>{\columncolor{greengreen}}c>{\columncolor{greengreen}}c} \toprule
    % {} & {} & {} & \multicolumn{2}{>{\columncolor{blueblue}}c}{Something-Something} \\
    {Method} & {Modalities at training} & {Modalities at inference} & {Views} & {Top 1} & {Top 5} \\ \midrule
    Baseline & RGB & RGB & 1x1 & 59.3 & 85.6 \\ \midrule
    Modality specific & OBJ & OBJ & 1x1 & 47.9 & 76.2 \\
    Teacher & \NA & RGB \& OBJ & 1x1 & X & X \\
    Student & RGB \& OBJ & RGB & 1x1 & 63.2\textsubscript{\textcolor{redred}{\textbf{+3.9}}} & 88.7\textsubscript{\textcolor{redred}{\textbf{+3.1}}} \\ \midrule
    Modality specific & OF & OF & 1x1 & 49.3 & 79.0 \\
    Teacher & \NA & RGB \& OF & 1x1 & X & X \\
    Student & RGB \& OF & RGB & 1x1 & 61.4\textsubscript{\textcolor{redred}{\textbf{+2.1}}} & 87.7\textsubscript{\textcolor{redred}{\textbf{+2.1}}} \\ \midrule
    Teacher & \NA & RGB \& OF \& OBJ & 1x1 & X & X \\
    % Omnivore \cite{bertasius2021space, girdhar2022omnivore} & RGB \& OF \& OD & RGB & 62.5 & 88.1 \\
    Student & RGB \& OF \& OBJ & RGB & 1x1 & 63.0\textsubscript{\textcolor{redred}{\textbf{+3.7}}} & 88.9\textsubscript{\textcolor{redred}{\textbf{+3.3}}} \\
    \bottomrule
\end{tabular}
}
\caption{Something-Something \cite{goyal2017something} object-agnostic action recognition.}
\end{subtable}
\caption{Epic-Kitchens \cite{damen2020rescaling} and Something-Something \cite{goyal2017something} ego-centric action recognition. Views = Spatial x Temporal crops; RGB = Video frames; OF = Optical flow; A = Audio; OBJ = Object detections. Teacher is ensemble (by logits average) of modality specific models. OBJ model is \cite{radevski2021revisiting}. Improvement over RGB frames baseline \cite{liu2021swin} (using same views) in \textbf{\textcolor{redred}{red}}.}
\end{table*}

\begin{table*}[t]
\begin{subtable}[t]{0.48\textwidth}
\centering
\resizebox{\columnwidth}{!}{
\begin{tabular}{>{\columncolor{graygray}}c>{\columncolor{pinkpink}}c>{\columncolor{yellowyellow}}c>{\columncolor{graygray}}c>{\columncolor{blueblue}}c>{\columncolor{blueblue}}c>{\columncolor{blueblue}}c} \toprule
    % {} & {} & \multicolumn{2}{|c|}{TT augmentation} & \multicolumn{3}{|c|}{Epic-100 Unseen} \\
    {Method} & {Training modalities} & {Inference Modalities} & {Views} & {Noun} & {Verb} & {Action} \\ \midrule
    Baseline & RGB & RGB & 1x1 & 38.3 & 51.7 & 25.4 \\ \midrule \midrule
    Modality specific & OF & OF & 1x1 & 28.0 & 53.2 & 21.6 \\
    Teacher & \NA & RGB \& OF & 1x1 & 41.0 & 54.9 & 28.4 \\
    Student & RGB \& OF & RGB & 1x1 & 42.5\textsubscript{\textcolor{redred}{\textbf{+4.2}}} & 55.9\textsubscript{\textcolor{redred}{\textbf{+4.2}}} & 30.2\textsubscript{\textcolor{redred}{\textbf{+4.8}}} \\ \midrule
    Modality specific & A & A & 1x1 & 15.0 & 41.5 & 9.1 \\
    Teacher & \NA & RGB \& A & 1x1 & 41.9 & 55.3 & 28.5 \\
    Student & RGB \& A & RGB & 1x1 & 41.8\textsubscript{\textcolor{redred}{\textbf{+3.5}}} & 51.8\textsubscript{\textcolor{redred}{\textbf{+0.1}}} & 27.5\textsubscript{\textcolor{redred}{\textbf{+2.1}}} \\ \midrule
  Teacher & \NA & RGB \& OF \& A & 1x1 & X & X & X \\
    Student & RGB \& OF \& A & RGB & 1x1 & 43.7\textsubscript{\textcolor{redred}{\textbf{+5.4}}} & 54.1\textsubscript{\textcolor{redred}{\textbf{+3.4}}} & 29.6\textsubscript{\textcolor{redred}{\textbf{+4.2}}} \\  \midrule \midrule \midrule
    Baseline & RGB & RGB & 3x4 & 43.1 & 54.4 & 29.1 \\ \midrule
    Modality specific & OF & OF & 3x4 & 31.6 & 54.9 & 23.5 \\
    Teacher & \NA & RGB \& OF & 3x4 & 43.9 & 56.5 & 30.1 \\
    Student & RGB \& OF & RGB & 3x4 & 44.5\textsubscript{\textcolor{redred}{\textbf{+1.4}}} & 56.9\textsubscript{\textcolor{redred}{\textbf{+2.5}}} & 30.5\textsubscript{\textcolor{redred}{\textbf{+1.4}}} \\ \midrule
    Baseline & RGB & RGB & 1x4 & 42.0 & 54.2 & 28.4 \\ \midrule \midrule \midrule
    Modality specific & A & A & 1x4 & 16.7 & 42.9 & 10.0 \\
  Teacher & \NA & RGB \& A & 1x4 & 44.2 & 57.6 & 31.1 \\
    Student & RGB \& A & RGB & 1x4 & 43.6\textsubscript{\textcolor{redred}{\textbf{+1.6}}} & 53.7\textsubscript{\textcolor{redred}{\textbf{-0.5}}} & 29.7\textsubscript{\textcolor{redred}{\textbf{+1.3}}} \\ \midrule
    Teacher & \NA & RGB \& OF \& A & 1x4 & X & X & X \\
    Student & RGB \& OF \& A & RGB & 1x4 & 44.4\textsubscript{\textcolor{redred}{\textbf{+2.4}}} & 57.2\textsubscript{\textcolor{redred}{\textbf{+3.2}}} & 30.9\textsubscript{\textcolor{redred}{\textbf{+2.5}}} \\ \bottomrule
\end{tabular}
}
\caption{Epic-Kitchens \cite{damen2020rescaling} active object (noun) and activity (verb) recognition \textit{strictly} on participants unseen during training).}
\end{subtable}
\hfill
\begin{subtable}[t]{0.48\textwidth}
\centering
\resizebox{\columnwidth}{!}{
\begin{tabular}{>{\columncolor{graygray}}c>{\columncolor{pinkpink}}c>{\columncolor{yellowyellow}}c>{\columncolor{graygray}}c>{\columncolor{blueblue}}c>{\columncolor{blueblue}}c} \toprule
    % {} & {} & {} & \multicolumn{2}{>{\columncolor{greengreen}}c}{Something-Else} \\
    {Method} & {Modalities at training} & {Modalities at inference} & {Views} & {Top 1} & {Top 5} \\ \midrule
    Baseline & RGB & RGB & 1x1 & 51.8 & 79.5 \\ \midrule
    Modality specific & OBJ & OBJ & 1x1 & 41.4 & 67.3 \\
    Teacher & \NA & RGB \& OBJ & 1x1 & X & X \\
    Student & RGB \& OBJ & RGB & 1x1 & 57.5\textsubscript{\textcolor{redred}{\textbf{+5.7}}} & 84.1\textsubscript{\textcolor{redred}{\textbf{4.6}}} \\ \midrule
    Modality specific & OF & OF & 1x1 & 49.0 & 77.4 \\
    Teacher & \NA & RGB \& OF & 1x1 & X & X \\
    Student & RGB \& OF & RGB & 1x1 & 56.2\textsubscript{\textcolor{redred}{\textbf{+4.4}}} & 83.7\textsubscript{\textcolor{redred}{\textbf{+4.2}}} \\ \midrule
    Teacher & \NA & RGB \& OF \& OBJ & 1x1 & X & X \\
    % Omnivore \cite{bertasius2021space, girdhar2022omnivore} & RGB \& OF \& OD & RGB & 56.8 & 83.3 \\
    Student & RGB \& OF \& OBJ & RGB & 1x1 & X\textsubscript{\textcolor{redred}{\textbf{+X}}} & X\textsubscript{\textcolor{redred}{\textbf{+X}}} \\
    \bottomrule
\end{tabular}
}
\caption{Something-Else \cite{materzynska2020something} (compositional split) object-agnostic action recognition where the object present at inference were unseen during training.}
\end{subtable}
\caption{Epic-Kitchens \cite{damen2020rescaling} (unseen split) and Something-Else\cite{materzynska2020something} (compositional split) ego-centric action recognition. Views = Spatial x Temporal crops; RGB = Video frames; OF = Optical flow; A = Audio; OBJ = Object detections. Teacher is ensemble (by logits average) of modality specific models. OBJ model is \cite{radevski2021revisiting}. Improvement over RGB frames baseline \cite{liu2021swin} (using same views) in \textbf{\textcolor{redred}{red}.}}
\end{table*}
