# Supplementary material for: Multimodal Distillation for Egocentric Action Recognition
Source: arXiv:2307.07483 source file (2023-07-18)
Supplement: Supplementary file 3 [file implementation.tex]

\section{Extended Implementation Details}\label{supp:implementation}
